# Supplementary material for: Effective Asymptotics of Combinatorial Systems
Source: arXiv:2508.20008 ancillary file (2025-08-27)
Supplement: Supplementary file 1 [file Examples_Section2.pdf]

## Examples from Section 2

Aug. 2025

These examples use generating functions instead of combinatorial objects because it is simpler with the tools provided by [combstruct](#). Still, the computations are exactly those that are presented at a combinatorial level in this section.

> **restart**

### Section 2.3 Characterization of Well-founded Systems by Leading Terms

#### Example 2

Fix the order on the variables to be as in the article

> **inds := [F, Tr, N1, N2, Tb, N3, Tg, N4, R, N5, N6, N7, B, N8, G, N9];**

*inds := [F, Tr, N1, N2, Tb, N3, Tg, N4, R, N5, N6, N7, B, N8, G, N9]*

Combinatorial system in the combstruct language (Union for +, Prod for \*)

> **combsys:={F=Set(Tr), Tr=Union(Z,N1), N1=Prod(R,N2), N2=Sequence(Tb), Tb=Prod(B,N3), N3=Sequence(Tg), Tg=Prod(G,N4), N4=Sequence(Tr), R=Union(N5,N6), N5=Prod(Z,Z,Z), N6=Prod(Z,N7), N7=Sequence(B), B=Prod(Z,N8), N8=Sequence(R), G=Union(Z,N9), N9=Prod(G,G)};**

*combsys := {B = Prod(Z, N8), F = Set(Tr), G = Union(Z, N9), N1 = Prod(R, N2), N2 = Sequence(Tb), N3 = Sequence(Tg), N4 = Sequence(Tr), N5 = Prod(Z, Z, Z), N6 = Prod(Z, N7), N7 = Sequence(B), N8 = Sequence(R), N9 = Prod(G, G), R = Union(N5, N6), Tb = Prod(B, N3), Tg = Prod(G, N4), Tr = Union(Z, N1)}*

Translation into generating function equations

> **sys:=combstruct[gfeqns](combsys, labelled, z);**

*sys := [B(z) = z N8(z), F(z) = e<sup>Tr(z)</sup>, G(z) = z + N9(z), N1(z) = R(z) N2(z), N2(z) =  $\frac{1}{1 - Tb(z)}$ , N3(z) =  $\frac{1}{1 - Tg(z)}$ , N4(z) =  $\frac{1}{1 - Tr(z)}$ , N5(z) = z<sup>3</sup>, N6(z) = z N7(z), N7(z) =  $\frac{1}{1 - B(z)}$ , N8(z) =  $\frac{1}{1 - R(z)}$ , N9(z) = G(z)<sup>2</sup>, R(z) = N5(z) + N6(z), Tb(z) = B(z) N3(z), Tg(z) = G(z) N4(z), Tr(z) = z + N1(z), Z(z) = z]*

> **sys:=subs([seq(i(z)=i, i=inds)], sys):**

Sort them in the order of the article:

```
> sys:=[seq(i=subs(sys,i),i=inds)];
```

$$\text{sys} := \left[ F = e^{Tr}, Tr = z + NI, NI = R N2, N2 = \frac{1}{1 - Tb}, Tb = B N3, N3 = \frac{1}{1 - Tg}, Tg = G N4, N4 = \frac{1}{1 - Tr}, R = N5 + N6, N5 = z^3, N6 = z N7, N7 = \frac{1}{1 - B}, B = z N8, N8 = \frac{1}{1 - R}, G = z + N9, N9 = G^2 \right]$$

Keep only the rhs for the iteration

```
> sys:=map2(op,2,sys):
```

Iterative computation of the leading terms:

```
> dim:=nops(inds):
```

```
> LTs:=[0$dim]:
```

```
> to dim+1 do LTs:=map(MultiSeries:-LeadingTerm,eval(sys,[seq(inds[i]=LTs[i],i=1..dim)]),z) until %=%%;
```

$$LTs := [1, z, 0, 1, 0, 1, 0, 1, 0, z^3, 0, 1, 0, 1, z, 0]$$

$$LTs := [1, z, 0, 1, 0, 1, z, 1, z^3, z^3, z, 1, z, 1, z, z^2]$$

$$LTs := [1, z, z^3, 1, z, 1, z, 1, z, z^3, z, 1, z, 1, z, z^2]$$

$$LTs := [1, z, z, 1, z, 1, z, 1, z, z^3, z, 1, z, 1, z, z^2]$$

$$LTs := [1, 2 z, z, 1, z, 1, z, 1, z, z^3, z, 1, z, 1, z, z^2]$$

$$LTs := [1, 2 z, z, 1, z, 1, z, 1, z, z^3, z, 1, z, 1, z, z^2]$$

### Example 3

```
> sys2:=subsop(-2=1+N9,-1=z*G^2,sys);
```

$$\text{sys2} := \left[ e^{Tr}, z + NI, R N2, \frac{1}{1 - Tb}, B N3, \frac{1}{1 - Tg}, G N4, \frac{1}{1 - Tr}, N5 + N6, z^3, z N7, \frac{1}{1 - B}, z N8, \frac{1}{1 - R}, 1 + N9, z G^2 \right]$$

```
> LTs:=[0$dim]:
```

```
> do LTs:=map(MultiSeries:-LeadingTerm,eval(sys2,[seq(inds[i]=LTs[i],i=1..dim)]),z) od;
```

$$LTs := [1, z, 0, 1, 0, 1, 0, 1, 0, z^3, 0, 1, 0, 1, 1, 0]$$

$$LTs := [1, z, 0, 1, 0, 1, 1, 1, z^3, z^3, z, 1, z, 1, 1, z]$$

Error, numeric exception: division by zero

This error detects that the system is not well-founded.

```
> sys3:=subs(1/(1-Tg)=(1+M,Tg*N3),sys2);
```

$$\text{sys3} := \left[ e^{Tr}, z + NI, R N2, \frac{1}{1 - Tb}, B N3, 1 + M, Tg N3, G N4, \frac{1}{1 - Tr}, N5 + N6, z^3, z N7, \right]$$

```


$$\left[ \frac{1}{1-B}, z^{N8}, \frac{1}{1-R}, 1 + N9, z^{G^2} \right]$$

> inds3:=subs(N3=(N3,M),inds);
      inds3 := [F, Tr, N1, N2, Tb, N3, M, Tg, N4, R, N5, N6, N7, B, N8, G, N9]
> dim3:=nops(inds3):
> LTs:=[0$dim3]:
> to dim3+1 do LTs:=map(MultiSeries:-LeadingTerm,eval(sys3,[seq(inds3
[i]=LTs[i],i=1..dim3)]),z) until %=%%;
      LTs := [1, z, 0, 1, 0, 1, 0, 0, 1, 0, z^3, 0, 1, 0, 1, 1, 0]
      LTs := [1, z, 0, 1, 0, 1, 0, 1, 1, z^3, z^3, z, 1, z, 1, 1, z]
      LTs := [1, z, z^3, 1, z, 1, 1, 1, 1, z, z^3, z, 1, z, 1, 1, z]
      LTs := [1, z, z, 1, z, 2, 1, 1, 1, z, z^3, z, 1, z, 1, 1, z]
      LTs := [1, 2 z, z, 1, 2 z, 2, 2, 1, 1, z, z^3, z, 1, z, 1, 1, z]
      LTs := [1, 2 z, z, 1, 2 z, 3, 2, 1, 1, z, z^3, z, 1, z, 1, 1, z]
      LTs := [1, 2 z, z, 1, 3 z, 3, 3, 1, 1, z, z^3, z, 1, z, 1, 1, z]
      LTs := [1, 2 z, z, 1, 3 z, 4, 3, 1, 1, z, z^3, z, 1, z, 1, 1, z]
      LTs := [1, 2 z, z, 1, 4 z, 4, 4, 1, 1, z, z^3, z, 1, z, 1, 1, z]
      LTs := [1, 2 z, z, 1, 4 z, 5, 4, 1, 1, z, z^3, z, 1, z, 1, 1, z]
      LTs := [1, 2 z, z, 1, 5 z, 5, 5, 1, 1, z, z^3, z, 1, z, 1, 1, z]
      LTs := [1, 2 z, z, 1, 5 z, 6, 5, 1, 1, z, z^3, z, 1, z, 1, 1, z]
      LTs := [1, 2 z, z, 1, 6 z, 6, 6, 1, 1, z, z^3, z, 1, z, 1, 1, z]
      LTs := [1, 2 z, z, 1, 6 z, 7, 6, 1, 1, z, z^3, z, 1, z, 1, 1, z]
      LTs := [1, 2 z, z, 1, 7 z, 7, 7, 1, 1, z, z^3, z, 1, z, 1, 1, z]
      LTs := [1, 2 z, z, 1, 7 z, 8, 7, 1, 1, z, z^3, z, 1, z, 1, 1, z]
      LTs := [1, 2 z, z, 1, 8 z, 8, 8, 1, 1, z, z^3, z, 1, z, 1, 1, z]
      LTs := [1, 2 z, z, 1, 8 z, 9, 8, 1, 1, z, z^3, z, 1, z, 1, 1, z]

```

The leading terms have not converged in a number of iterations equal to the dimension of the system. It is therefore not well founded.

## Section 2.4. Example 5

```

> combsys:={F=Set(Tr),Tr=Union(Z,Prod(R,Sequence(Tb))),Tb=Prod(B,
Sequence(Tg)),Tg=Prod(G,Sequence(Tr)),R=Union(Prod(Z,Z,Z),Prod(Z,
Sequence(B))),B=Prod(Z,Sequence(R)),G=Union(Z,Prod(G,G))};
combsys := {B = Prod(Z, Sequence(R)), F = Set(Tr), G = Union(Z, Prod(G, G)), R
= Union(Prod(Z, Z, Z), Prod(Z, Sequence(B))), Tb = Prod(B, Sequence(Tg)), Tg = Prod(G,
Sequence(Tr)), Tr = Union(Z, Prod(R, Sequence(Tb)))}
> inds:=[F,Tr,Tb,Tg,R,B,G]:

```

```
> sys:=comstruct[gfeqns](combsys,labelled,z):
```

```
> sys:=subs([seq(i(z)=i,i=inds)],sys):
```

Sort them in the order of the article:

```
> sys:=[seq(i=subs(sys,i),i=inds)];
```

$$\text{sys} := \left[ F = e^{Tr}, Tr = z + \frac{R}{1 - Tb}, Tb = \frac{B}{1 - Tg}, Tg = \frac{G}{1 - Tr}, R = z^3 + \frac{z}{1 - B}, B = \frac{z}{1 - R}, G = G^2 + z \right]$$

This is the generating function version of the combinatorial Jacobian matrix of that system

```
> VectorCalculus['Jacobian'](map(rhs,sys),inds);
```

$$\begin{bmatrix} 0 & e^{Tr} & 0 & 0 & 0 & 0 & \dots \\ 0 & 0 & \frac{R}{(1 - Tb)^2} & 0 & \frac{1}{1 - Tb} & 0 & \dots \\ 0 & 0 & 0 & \frac{B}{(1 - Tg)^2} & 0 & \frac{1}{1 - Tg} & \dots \\ 0 & \frac{G}{(1 - Tr)^2} & 0 & 0 & 0 & 0 & \dots \\ 0 & 0 & 0 & 0 & 0 & \frac{z}{(1 - B)^2} & \dots \\ 0 & 0 & 0 & 0 & \frac{z}{(1 - R)^2} & 0 & \dots \\ 0 & 0 & 0 & 0 & 0 & 0 & \dots \end{bmatrix}$$
