# Supplementary material for: Effective Asymptotics of Combinatorial Systems
Source: arXiv:2508.20008 ancillary file (2025-08-27)
Supplement: Supplementary file 2 [file MainExample.pdf]

# Main Example

Aug. 2025

This worksheet gives details of the computations around the combinatorial specification introduced in Section 2.2 and used in many of the examples of the article.

> **restart**

Parts of this worksheet use the package NewtonGF, that can be downloaded from

<https://perso.ens-lyon.fr/bruno.salvy/software/the-newtongf-package/>

> **with(NewtonGF);**

[*BoltzmannExpectedSize, BoltzmannParameter, GFSeries, NumericalNewtonIteration, Radius, SeriesNewtonIteration*]

> **NewtonGF:-version;**

2.21

Short procedures to compute Jacobian and Hessian

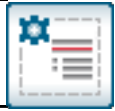

**jac:=proc(sys,inds) VectorCalculus[Jacobian](args) end:**

## Combinatorial Equations (Example 1)

Combinatorial system of equation (4)

> **combsys:=[F=Set(Tr),Tr=Union(Z,Prod(R,Sequence(Tb))),Tb=Prod(B,Sequence(Tg)),Tg=Prod(G,Sequence(Tr)),R=Union(Prod(Z,Z,Z),Prod(Z,Sequence(B))),B=Prod(Z,Sequence(R)),G=Union(Z,Prod(G,G))];**

*combsys := [F = Set(Tr), Tr = Union(Z, Prod(R, Sequence(Tb))), Tb = Prod(B, Sequence(Tg)),  
Tg = Prod(G, Sequence(Tr)), R = Union(Prod(Z, Z, Z), Prod(Z, Sequence(B))), B = Prod(Z,  
Sequence(R)), G = Union(Z, Prod(G, G))]*

Its indeterminates in the same order as in the article

> **inds:=map2(op,1,combsys);**

*inds := [F, Tr, Tb, Tg, R, B, G]*

Number of unknowns

> **dim:=nops(inds);**

*dim := 7*

## Generating Function Equations (Example 13)

The command `combstruct[gfeqns]` computes generating function equations

```
> gfsys:=combstruct[gfeqns]({op(combsys)},labeled,z):
```

Change order to reflect inds and replace f(z) by f for all f.

```
> gfsys:=subs(seq(i(z)=i,i=inds),[seq(i(z)=subs(gfsys,i(z)),i=inds)])
;
```

$$gfsys := \left[ F = e^{Tr}, Tr = z + \frac{R}{1 - Tb}, Tb = \frac{B}{1 - Tg}, Tg = \frac{G}{1 - Tr}, R = z^3 + \frac{z}{1 - B}, B = \frac{z}{1 - R}, G = G^2 + z \right]$$

## Newton Iteration and Newton-Kantorovich Bound (Example 15)

System of generating function equations

```
> sys:=[seq(op(1,i)-op(2,i),i=gfsys)];
```

$$sys := \left[ F - e^{Tr}, Tr - z - \frac{R}{1 - Tb}, Tb - \frac{B}{1 - Tg}, Tg - \frac{G}{1 - Tr}, R - z^3 - \frac{z}{1 - B}, B - \frac{z}{1 - R}, -G^2 + G - z \right]$$

Its Jacobian matrix

```
> J:=jac(sys,inds);
J:=
```

$$\begin{bmatrix}
 1 & -e^{Tr} & 0 & 0 & 0 & \dots \\
 0 & 1 & -\frac{R}{(1-Tb)^2} & 0 & -\frac{1}{1-Tb} & \dots \\
 0 & 0 & 1 & -\frac{B}{(1-Tg)^2} & 0 & \dots \\
 0 & -\frac{G}{(1-Tr)^2} & 0 & 1 & 0 & \dots \\
 0 & 0 & 0 & 0 & 1 & \dots \\
 0 & 0 & 0 & 0 & -\frac{z}{(1-R)^2} & \dots \\
 0 & 0 & 0 & 0 & 0 & \dots
 \end{bmatrix}$$

Two procedures: one that returns the first iterates of Newton's iteration started at 0; another one that takes that input and checks whether an upper bound on the distance to the solution can be computed by the Newton-Kantorovich bound.

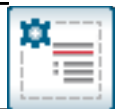

```
newtit:=proc(sys,vars,z,Jac,a,nbit)
```

```
> a:=.1703915;
```

```
a := 0.1703915
```

First 15 iterations starting from 0 at z=a:

```
> L:=newtit(sys,inds,z,J,a,15);
```

$$L := \left[ \begin{array}{c} \left[ \begin{array}{c} 0 \\ 0 \\ 0 \\ 0 \\ 0 \\ 0 \\ 0 \end{array} \right], \left[ \begin{array}{c} 1.38087428663078 \\ 0.380874286630778 \\ 0.206255977738198 \\ 0.170391500000000 \\ 0.210482786630778 \\ 0.206255977738198 \\ 0.170391500000000 \end{array} \right], \left[ \begin{array}{c} 1.62845257711394 \\ 0.493536949389897 \\ 0.332052410869526 \\ 0.396429637531613 \\ 0.223136427733548 \\ 0.219276251555321 \\ 0.214433542714690 \end{array} \right] \end{array} \right],$$

$$\left[ \begin{array}{c} \left[ \begin{array}{c} 1.71880185500292 \\ 0.542802561863069 \\ 0.408486506223766 \\ 0.471285228566121 \\ 0.223217284646040 \\ 0.219355419200494 \\ 0.217829777596269 \end{array} \right], \left[ \begin{array}{c} 1.76270985750583 \\ 0.567143844424058 \\ 0.438873629475690 \\ 0.501856523894911 \\ 0.223217287804178 \\ 0.219355422468575 \\ 0.217850216342911 \end{array} \right] \end{array} \right],$$

$$\left[ \begin{array}{c} \left[ \begin{array}{c} 1.78264626995608 \\ 0.578159155486607 \\ 0.452930608443642 \\ 0.516093072208912 \\ 0.223217287804178 \\ 0.219355422468575 \\ 0.217850217083195 \end{array} \right], \left[ \begin{array}{c} 1.79219061833084 \\ 0.583452641984251 \\ 0.459684676129003 \\ 0.522907921328802 \\ 0.223217287804178 \\ 0.219355422468575 \\ 0.217850217083195 \end{array} \right] \end{array} \right],$$

1.79684501391378  
0.586035687283299  
0.462980624796294  
0.526233381234724  
0.223217287804178  
0.219355422468575  
0.217850217083195

1.79910640633699  
0.587290887816237  
0.464582322139187  
0.527849295680426  
0.223217287804178  
0.219355422468575  
0.217850217083195

1.80015134334517  
0.587870909151187  
0.465322465354405  
0.528595994880922  
0.223217287804178  
0.219355422468575  
0.217850217083195

1.80054634202999  
0.588090166231539  
0.465602251747425  
0.528878258212049  
0.223217287804178  
0.219355422468575  
0.217850217083195

1.80062576655116  
0.588134253542321  
0.465658510081802  
0.528935014531359  
0.223217287804178  
0.219355422468575  
0.217850217083195

1.80062926497161  
0.588136195461976  
0.465660988100577  
0.528937514484209  
0.223217287804178  
0.219355422468575  
0.217850217083195

$$\begin{bmatrix} 1.80062927178705 \\ 0.588136199245125 \\ 0.465660992928127 \\ 0.528937519354490 \\ 0.223217287804178 \\ 0.219355422468575 \\ 0.217850217083195 \end{bmatrix}, \begin{bmatrix} 1.80062927178707 \\ 0.588136199245135 \\ 0.465660992928140 \\ 0.528937519354503 \\ 0.223217287804178 \\ 0.219355422468575 \\ 0.217850217083195 \end{bmatrix}, \\
 \begin{bmatrix} 1.80062927178708 \\ 0.588136199245141 \\ 0.465660992928147 \\ 0.528937519354510 \\ 0.223217287804178 \\ 0.219355422468575 \\ 0.217850217083195 \end{bmatrix}$$

Vector constructed from the Hessian matrices of the coordinates of the system in Thm. 4.4

**> Hess:=hessian(sys,inds);**

$$\begin{aligned}
Hess := & \begin{bmatrix}
-e^{Tr} \\
-\frac{2R}{(1-Tb)^3} - \frac{2}{(1-Tb)^2} \\
-\frac{2B}{(1-Tg)^3} - \frac{2}{(1-Tg)^2} \\
-\frac{2G}{(1-Tr)^3} - \frac{2}{(1-Tr)^2} \\
-\frac{2z}{(1-B)^3} \\
-\frac{2z}{(1-R)^3} \\
-2
\end{bmatrix}
\end{aligned}$$

Newton-Kantorovich test for each of the iterations in L: either it fails because the hypotheses of Thm. 4.4 do not apply (then it reports which one), or it returns a distance to the solution

```

> for i from 2 to nops(L) do i,checklast(sys,inds,z,J,Hess,a,L[1..i])
od;

```

```

      2, FAIL, "step larger than coordinate"
      3, FAIL, "step larger than coordinate"
      4, FAIL, "inequality not satisfied", 102.808030151466042, 0.1806985558
      5, FAIL, "inequality not satisfied", 164.991706949433421, 0.08781600502
      6, FAIL, "inequality not satisfied", 287.614470625521392, 0.03987282492
      7, FAIL, "inequality not satisfied", 545.300112200975036, 0.01908869675
      8, FAIL, "inequality not satisfied", 1062.55121137258743, 0.009308791166
      9, FAIL, "inequality not satisfied", 2081.24418068090881, 0.004522784848
     10, FAIL, "inequality not satisfied", 3989.52438469536401, 0.002089874018
     11, FAIL, "inequality not satisfied", 6986.71435337255571, 0.0007899973698
     12, FAIL, "inequality not satisfied", 9778.72086969745033, 0.0001588490424
     13, 5.712920594 × 10-6
     14, 1.112962112 × 10-8
     15, 2.900790719 × 10-14
     16, 1.704214548 × 10-14

```

At a larger starting point b, the iteration does not converge, showing that b is larger than the radius of convergence.

```
> b:=0.1703918:
> L:=newtit(sys,inds,z,J,b,15):
negative step at 12 th iteration: -0.0009996
negative step at 13 th iteration: -0.00078947
negative step at 15 th iteration: -0.00109508
```

## Radius of convergence and values at that point (Example 18)

Split the system by connected components:

```
> comp:=[[G],[B,R],[Tr,Tb,Tg],[F]];
      comp := [[G], [B, R], [Tr, Tb, Tg], [F]]
```

```
> for cc in comp do
  Sys[cc]:=[seq(i-subs(gfsys,i),i=cc)]
od;
```

$$Sys_{[G]} := [-G^2 + G - z]$$

$$Sys_{[B,R]} := \left[ B - \frac{z}{1-R}, R - z^3 - \frac{z}{1-B} \right]$$

$$Sys_{[Tr,Tb,Tg]} := \left[ Tr - z - \frac{R}{1-Tb}, Tb - \frac{B}{1-Tg}, Tg - \frac{G}{1-Tr} \right]$$

$$Sys_{[F]} := [F - e^{Tr}]$$

Newton iteration for a characteristic system

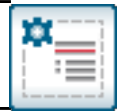

```
newtcharsys:=proc(sys,vars,ini,nbit) # Prototype, should be rew
```

## First component G

```
> cc:=comp[1];
```

$$cc := [G]$$

Its Jacobian matrix

```
> J:=jac(Sys[cc],cc);
```

$$J := \begin{bmatrix} -2G + 1 \end{bmatrix}$$

the characteristic system

```
> charsys:=[op(Sys[cc]),LinearAlgebra[Determinant](J)];
```

$$charsys := [-G^2 + G - z, -2G + 1]$$

Use Newton iteration at a point to find a starting point for a Newton iteration on the characteristic system

```
> a:=.01:L:=newtit(Sys[cc],cc,z,J,a,8);
```

$$L := \begin{bmatrix} \begin{bmatrix} 0 \end{bmatrix}, \begin{bmatrix} 0.010000000000000000 \end{bmatrix}, \begin{bmatrix} 0.0101020408163265 \end{bmatrix}, \\ \begin{bmatrix} 0.0101020514433643 \end{bmatrix}, \begin{bmatrix} 0.0101020514433644 \end{bmatrix}, \\ \begin{bmatrix} 0.0101020514433644 \end{bmatrix}, \begin{bmatrix} 0.0101020514433644 \end{bmatrix}, \\ \begin{bmatrix} 0.0101020514433644 \end{bmatrix}, \begin{bmatrix} 0.0101020514433644 \end{bmatrix} \end{bmatrix}$$

```
> H:=hessian(Sys[cc],cc);
```

$$H := \begin{bmatrix} -2 \end{bmatrix}$$

Newton-Kantorovich test:

```
> checklast(Sys[cc],cc,z,J,H,a,L);
```

$$1.897978302 \times 10^{-16}$$

Thus this point is inside the domain of convergence. Use it at a starting point to find the radius of convergence

```
> newtcharsys(charsys,[op(cc),z],[L[-1][1],a],3);
```

$$\begin{bmatrix} \begin{bmatrix} 0.0101020514433644 \\ 0.01 \end{bmatrix}, \begin{bmatrix} 0.5000000000000000 \\ 0.4900000000000000 \end{bmatrix}, \\ \begin{bmatrix} 0.5000000000000000 \\ 0.2500000000000000 \end{bmatrix}, \begin{bmatrix} 0.5000000000000000 \\ 0.2500000000000000 \end{bmatrix} \end{bmatrix}$$

The radius of convergence for that component is 1/4, and G=1/2 there.

## Second component B,R

Same computations

```
> cc:=comp[2];
```

$$cc := [B, R]$$

```
> J:=jac(Sys[cc],cc);
```

$$J := \begin{bmatrix} 1 & -\frac{z}{(1-R)^2} \\ -\frac{z}{(1-B)^2} & 1 \end{bmatrix}$$

```
> charsys:=[op(Sys[cc]),LinearAlgebra[Determinant](J)];
```

$$\text{charsys} := \left[ B - \frac{z}{1-R}, R - z^3 - \frac{z}{1-B}, \frac{B^2 R^2 - 2 B^2 R - 2 B R^2 + B^2 + 4 B R + R^2 - z^2 - 2 B - 2 R + 1}{(-1+R)^2 (-1+B)^2} \right]$$

> **a:=.1:L:=newtit(Sys[cc],cc,z,J,a,6);**

$$L := \left[ \begin{bmatrix} 0 \\ 0 \end{bmatrix}, \begin{bmatrix} 0.111212121212121 \\ 0.112121212121212 \end{bmatrix}, \begin{bmatrix} 0.112830496483439 \\ 0.113717657723301 \end{bmatrix}, \begin{bmatrix} 0.112830915619644 \\ 0.113718084704026 \end{bmatrix}, \begin{bmatrix} 0.112830915619674 \\ 0.113718084704054 \end{bmatrix}, \begin{bmatrix} 0.112830915619674 \\ 0.113718084704054 \end{bmatrix} \right]$$

> **H:=hessian(Sys[cc],cc);**

$$H := \begin{bmatrix} -\frac{2z}{(1-R)^3} \\ -\frac{2z}{(1-B)^3} \end{bmatrix}$$

> **checklast(Sys[cc],cc,z,J,H,a,L);**

$$4.879220640 \times 10^{-14}$$

The values are correct at that point, but it turns out that it is too far for Newton's iteration on the characteristic system to converge:

> **newtcharsys(charsys,[op(cc),z],[L[-1][1..nops(cc)],a],5);**

$$\left[ \begin{bmatrix} 0.112830915619674 \\ 0.113718084704054 \\ 0.1 \end{bmatrix}, \begin{bmatrix} 3.15707140771906 \\ 3.21740289883661 \\ 2.44786369458586 \end{bmatrix}, \begin{bmatrix} -0.690384761113947 \\ 3.64110863527104 \\ 1.99860381221222 \end{bmatrix}, \begin{bmatrix} -3.54368806339087 \\ -7.64244495504647 \\ 0.820671571099570 \end{bmatrix} \right]$$

$$\begin{bmatrix} 106.454811838973 \\ 1701.11749854816 \\ 757.768973403106 \end{bmatrix}, \begin{bmatrix} -12422.3939246206 \\ -4.73806415951467 \times 10^7 \\ 477.675168808094 \end{bmatrix}$$

Pick a larger value for a and compute a new starting point

```
> a:=.15:L:=newtit(Sys[cc],cc,z,J,a,5):
> checklast(Sys[cc],cc,z,J,H,a,L);
```

$$4.532485498 \times 10^{-17}$$

This is still too far:

```
> newtcharsys(charsys,[op(cc),z],[L[-1][1..nops(cc)],a],5);
```

$$\begin{bmatrix} \begin{bmatrix} 0.184576418731544 \\ 0.187328473318325 \\ 0.15 \end{bmatrix} \\ \begin{bmatrix} 0.924859056120317 \\ 6.86730695005865 \\ 7.97349405298648 \end{bmatrix} \\ \begin{bmatrix} 0.954022506395547 \\ 1840.99044203594 \\ 581.142061743403 \end{bmatrix} \end{bmatrix}, \begin{bmatrix} \begin{bmatrix} 1.57805792640201 \\ 1.62384389259156 \\ 1.01729587269914 \end{bmatrix} \\ \begin{bmatrix} 1.01888093714952 \\ 14.4961255200565 \\ 4.38924827341878 \end{bmatrix} \\ \begin{bmatrix} 1.14403868192165 \\ 9732.32859116484 \\ 387.377773070472 \end{bmatrix} \end{bmatrix},$$

An even larger value for a:

```
> a:=.2:L:=newtit(Sys[cc],cc,z,J,a,5):
> checklast(Sys[cc],cc,z,J,H,a,L);
```

$$1.600873878 \times 10^{-13}$$

Now we have convergence:

```
> newtcharsys(charsys,[op(cc),z],[L[-1][1..nops(cc)],a],11);
```

$$\begin{bmatrix} \begin{bmatrix} 0.280029327467970 \\ 0.285789092848226 \\ 0.2 \end{bmatrix} \\ \begin{bmatrix} 0.845585922815373 \\ 0.867641993519010 \\ 0.440990812548610 \end{bmatrix} \end{bmatrix}, \begin{bmatrix} \begin{bmatrix} 0.845585922815373 \\ 0.867641993519010 \\ 0.440990812548610 \end{bmatrix} \end{bmatrix},$$

$$\begin{bmatrix} 0.882078429509694 \\ 0.886400137892187 \\ 0.0542516994490947 \end{bmatrix}, \begin{bmatrix} 0.757573401480074 \\ 0.759393986939897 \\ 0.146714352724428 \end{bmatrix}, \\
 \begin{bmatrix} 0.642504945924119 \\ 0.645373584538174 \\ 0.224116785622729 \end{bmatrix}, \begin{bmatrix} 0.561067712327155 \\ 0.567082442535303 \\ 0.248447863951680 \end{bmatrix}, \\
 \begin{bmatrix} 0.515014505279682 \\ 0.522381088307625 \\ 0.248612565179414 \end{bmatrix}, \begin{bmatrix} 0.501115867127810 \\ 0.508591796419913 \\ 0.246520085705599 \end{bmatrix}, \\
 \begin{bmatrix} 0.500006927065988 \\ 0.507474683169243 \\ 0.246267917400333 \end{bmatrix}, \begin{bmatrix} 0.500000000276904 \\ 0.507467655946209 \\ 0.246266172238312 \end{bmatrix}, \\
 \begin{bmatrix} 0.500000000000000 \\ 0.507467655664555 \\ 0.246266172167723 \end{bmatrix}, \begin{bmatrix} 0.500000000000000 \\ 0.507467655664555 \\ 0.246266172167723 \end{bmatrix}$$

Here are the lengths of the Newton steps:

**> seq(%[i+1]-%[i],i=1..nops(%)-1);**

$$\begin{bmatrix} 0.565556595347403 \\ 0.581852900670784 \\ 0.240990812548610 \end{bmatrix}, \begin{bmatrix} 0.0364925066943210 \\ 0.0187581443731772 \\ -0.386739113099516 \end{bmatrix}, \\
 \begin{bmatrix} -0.124505028029620 \\ -0.127006150952290 \\ 0.0924626532753338 \end{bmatrix}, \begin{bmatrix} -0.115068455555955 \\ -0.114020402401723 \\ 0.0774024328983003 \end{bmatrix},$$

$$\begin{bmatrix} -0.0814372335969644 \\ -0.0782911420028712 \\ 0.0243310783289510 \end{bmatrix}, \begin{bmatrix} -0.0460532070474731 \\ -0.0447013542276781 \\ 0.000164701227733793 \end{bmatrix}, \\
\begin{bmatrix} -0.0138986381518715 \\ -0.0137892918877117 \\ -0.00209247947381494 \end{bmatrix}, \begin{bmatrix} -0.00110894006182216 \\ -0.00111711325066999 \\ -0.000252168305265255 \end{bmatrix}, \\
\begin{bmatrix} -6.92678908342792 \times 10^{-6} \\ -7.02722303425052 \times 10^{-6} \\ -1.74516202175456 \times 10^{-6} \end{bmatrix}, \\
\begin{bmatrix} -2.76904055240834 \times 10^{-10} \\ -2.81654255473995 \times 10^{-10} \\ -7.05889513508140 \times 10^{-11} \end{bmatrix}, \\
\begin{bmatrix} -3.88578058618805 \times 10^{-16} \\ -3.33066907387547 \times 10^{-16} \\ 0. \end{bmatrix}$$

Evaluation at  $a < \rho$  gives a lower bound on the values of  $B(\rho), R(\rho)$ :

**> newtit(Sys[cc], cc, z, J, .2462661, 5);**

$$\begin{bmatrix} \begin{bmatrix} 0 \\ 0 \end{bmatrix}, \begin{bmatrix} 0.330643695163086 \\ 0.342627731397402 \end{bmatrix}, \begin{bmatrix} 0.428057276331103 \\ 0.436393940620996 \end{bmatrix}, \\
\begin{bmatrix} 0.466390721979440 \\ 0.474372296453242 \end{bmatrix}, \begin{bmatrix} 0.483743598150439 \\ 0.491453677883130 \end{bmatrix}, \\
\begin{bmatrix} 0.491999296668785 \\ 0.499586444281971 \end{bmatrix} \end{bmatrix}$$

```
> checklast(Sys[cc],cc,z,J,H,.2462661,L);
1.600873878 × 10-13
```

### Third component Tr,Tb,Tg

Same computations:

```
> cc:=map(op,comp[1..3]);
cc := [G, B, R, Tr, Tb, Tg]
```

```
> newsys:=map(op,[seq(Sys[comp[i]],i=1..3)]);
```

```
newsys := [ -G2 + G - z, B -  $\frac{z}{1-R}$ , R - z3 -  $\frac{z}{1-B}$ , Tr - z -  $\frac{R}{1-Tb}$ , Tb -  $\frac{B}{1-Tg}$ , Tg
-  $\frac{G}{1-Tr}$  ]
```

```
> J:=jac(newsys,cc);
```

```
J :=
```

$$\begin{bmatrix} -2G + 1 & 0 & 0 & 0 & \dots \\ 0 & 1 & -\frac{z}{(1-R)^2} & 0 & \dots \\ 0 & -\frac{z}{(1-B)^2} & 1 & 0 & \dots \\ 0 & 0 & -\frac{1}{1-Tb} & 1 & -\frac{1}{1-Tg} \\ 0 & -\frac{1}{1-Tg} & 0 & 0 & \dots \\ -\frac{1}{1-Tr} & 0 & 0 & -\frac{G}{(1-Tr)^2} & \dots \end{bmatrix}$$

```
> charsys:=[op(newsys),LinearAlgebra[Determinant](J)];
```

```
charsys := [ -G2 + G - z, B -  $\frac{z}{1-R}$ , R - z3 -  $\frac{z}{1-B}$ , Tr - z -  $\frac{R}{1-Tb}$ , Tb -  $\frac{B}{1-Tg}$ , Tg
-  $\frac{G}{1-Tr}$ , -(( -2G + 1) (B2 R2 - 2B2 R - 2BR2 + B2 + 4BR + R2 - z2 - 2B
- 2R + 1) (-Tb2 Tg2 Tr2 + 2Tb2 Tg2 Tr + 2Tb2 Tg Tr2 + 2Tb Tg2 Tr2 - Tb2 Tg2
```

$$\begin{aligned}
 & -4 Tb^2 Tg Tr - Tb^2 Tr^2 - 4 Tb Tg^2 Tr - 4 Tb Tg Tr^2 - Tg^2 Tr^2 + G R B + 2 Tb^2 Tg \\
 & + 2 Tb^2 Tr + 2 Tb Tg^2 + 8 Tb Tg Tr + 2 Tb Tr^2 + 2 Tg^2 Tr + 2 Tg Tr^2 - Tb^2 - 4 Tb Tg \\
 & - 4 Tb Tr - Tg^2 - 4 Tg Tr - Tr^2 + 2 Tb + 2 Tg + 2 Tr - 1) \Big/ ((-1 + R)^2 (-1 \\
 & + B)^2 (-1 + Tr)^2 (-1 + Tb)^2 (-1 + Tg)^2) ]
 \end{aligned}$$

> a:=.16:L:=newtit(newsys,cc,z,J,a,7):

> H:=hessian(newsys,cc):

> checklast(newsys,cc,z,J,H,a,L);

$9.064970999 \times 10^{-17}$

> newtcharsys(charsys,[op(cc),z],[L[-1][1..nops(cc)],a],10);

|                    |                   |
|--------------------|-------------------|
| 0.2000000000000000 | 0.270083008482840 |
| 0.201098771154914  | 0.272600177594664 |
| 0.204371070588263  | 0.278159598892876 |
| 0.460327630133616  | 0.731808544697085 |
| 0.319506265549598  | 0.593666535597532 |
| 0.370595218816775  | 0.686884410094676 |
| 0.16               | 0.202049805089704 |
| 0.216334950427360  | 0.217944979327467 |
| 0.216388764587936  | 0.219465901838193 |
| 0.220194952183885  | 0.223329407285527 |
| 0.689153169546069  | 0.641632171251337 |
| 0.578722351119142  | 0.531217785877908 |
| 0.646473717453715  | 0.594738483639488 |
| 0.172422993395687  | 0.170447557506476 |

0.219159433987173

0.220698014436811

0.224603476537946

0.607115876902765

0.488772499075064

0.552973756184335

0.171130051381716

0.218205065725156

0.219719167814966

0.223592842538241

0.591313461204765

0.469405493166660

0.532956455130208

0.170592525835816

0.217860478332407

0.219365925344204

0.223228131310148

0.588694405375917

0.466363155679739

0.529653161898660

0.170397409053653

0.217850526504527

0.219355739740976

0.223217615378514

0.588633469593621

0.466295302955215

0.529577649482338

0.170391674705267

0.217850521102699

0.219355734219893

0.223217609678839

0.588633437777379

0.466295268173328

0.529577610600257

0.170391671557982

0.217850521102698

0.219355734219891

0.223217609678837

0.588633437777368

0.466295268173315

0.529577610600243

0.170391671557981

```

0.217850521102698
0.219355734219891
0.223217609678837
0.588633437777371
0.466295268173319
0.529577610600248
0.170391671557981

```

Lengths of the Newton steps on the characteristic system:

```
> seq(%[i+1]-%[i],i=1..nops(%)-1);
```

```

0.0700830084828404      -0.0537480580554803
0.0715014064397497      -0.0562114130067272
0.0737885283046130      -0.0579646467089911
0.271480914563469      -0.0426553751510161
0.274160270047935      -0.0149441844783907
0.316289191277902      -0.0404106926409612
0.0420498050897042      -0.0296268116940172

```

```

0.00161002890010656      0.00121445465970665
0.00307713725025699      0.00123211259861788
0.00313445510164198      0.00127406925241902
-0.0475209982947320      -0.0345162943485717
-0.0475045652412339      -0.0424452868028437
-0.0517352338142275      -0.0417647274551525
-0.00197543588921106      0.000682493875239637

```

−0.000954368262017669

−0.000978846621844970

−0.00101063399970530

−0.0158024156980004

−0.0193670059084038

−0.0200173010541270

−0.000537525545899920

−0.000344587392748591

−0.000353242470761933

−0.000364711228093451

−0.00261905582884758

−0.00304233748692123

−0.00330329323154788

−0.000195116782162608

−9.95182787957849 × 10<sup>−6</sup>

−0.0000101856032288239

−0.0000105159316332037

−0.0000609357822960455

−0.0000678527245238647

−0.0000755124163224208

−5.73434838654907 × 10<sup>−6</sup>

−5.40182831798575 × 10<sup>−9</sup>

−5.52108289642028 × 10<sup>−9</sup>

−5.69967564811868 × 10<sup>−9</sup>

−3.18162418633250 × 10<sup>−8</sup>

−3.47818876478279 × 10<sup>−8</sup>

−3.88820809993362 × 10<sup>−8</sup>

−3.14728490491412 × 10<sup>−9</sup>

$$\begin{bmatrix} -1.44328993201270 \times 10^{-15} \\ -1.49880108324396 \times 10^{-15} \\ -1.52655665885959 \times 10^{-15} \\ -1.09912079437890 \times 10^{-14} \\ -1.23789867245705 \times 10^{-14} \\ -1.34336985979644 \times 10^{-14} \\ -8.60422844084496 \times 10^{-16} \end{bmatrix}, \begin{bmatrix} 0. \\ 0. \\ 0. \\ 3.21964677141295 \times 10^{-15} \\ 4.16333634234434 \times 10^{-15} \\ 4.21884749357559 \times 10^{-15} \\ 0. \end{bmatrix}$$

The radius of convergence has been found, together with the values of the generating functions there:

```
> vals:=[seq(cc[i]=%%[-1][i],i=1..nops(cc)),rho=%%[-1][-1]];
vals := [G = 0.217850521102698, B = 0.219355734219891, R = 0.223217609678837, Tr
= 0.588633437777371, Tb = 0.466295268173319, Tg = 0.529577610600248, p
= 0.170391671557981]
```

Evaluation at  $a < \rho$  gives a lower bound on the values of all coordinates at  $\rho$ :

```
> newtit(newsys,cc,z,J,.1703916,10);
```

$$\begin{bmatrix} 0 \\ 0 \\ 0 \\ 0 \\ 0 \\ 0 \end{bmatrix}, \begin{bmatrix} 0.170391600000000 \\ 0.206256125100897 \\ 0.210482941065742 \\ 0.380874541065742 \\ 0.206256125100897 \\ 0.170391600000000 \end{bmatrix}, \begin{bmatrix} 0.214433707771768 \\ 0.219276432734236 \\ 0.223136614802749 \\ 0.493537490449076 \\ 0.332052877755952 \\ 0.396430244427670 \end{bmatrix},$$

0.217829954649935

0.219355600918010

0.223217472264010

0.542803663601189

0.408487776437260

0.471286626053459

0.217850393553794

0.219355604186141

0.223217475422196

0.567146134209432

0.438876408679642

0.501859440673454

0.217850394294091

0.219355604186141

0.223217475422196

0.578163799038738

0.452936394678697

0.516099026674841

0.217850394294091

0.219355604186141

0.223217475422196

0.583461988505799

0.459696465094042

0.522919931793514

0.217850394294091

0.219355604186141

0.223217475422196

0.586054395196344

0.463004360104278

0.526257444115364

0.217850394294091

0.219355604186141

0.223217475422196

0.587327972454666

0.464629507668284

0.527897016499404

```

0.217850394294091
0.219355604186141
0.223217475422196
0.587942149706189
0.465413236256464
0.528687686925677

```

```

0.217850394294091
0.219355604186141
0.223217475422196
0.588213392607796
0.465759360096832
0.529036874891572

```

```

> checklast(newsys,cc,z,J,H,.1703916,L); # bound on the distance to
the value

```

$$9.064970999 \times 10^{-17}$$

## Last component F

```

> F=subs(gfsys,F);

```

$$F = e^{Tr}$$

Since this is an exponential, its singularities are those of its argument.

```

> eval(%,vals);

```

$$F = 1.80152483667951$$

```

> vals:=[op(vals),%];

```

```

vals := [G = 0.217850521102698, B = 0.219355734219891, R = 0.223217609678837, Tr
= 0.588633437777371, Tb = 0.466295268173319, Tg = 0.529577610600248, ρ
= 0.170391671557981, F = 1.80152483667951 ]

```

## Expansions at the Dominant Singularity (Section 8.4)

The following procedure is an optimization: it computes orders for Newton iteration over power series that avoid overshooting with powers of 2

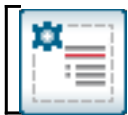

```

newtords:=proc(k)

```

## Expansion of G,B,R

Change this variable to compute more terms in the expansion

```

> nbterms:=4;

```

$$nbterms := 4$$

```

> eq:=op(Sys[[G]]);

```

$$eq := -G^2 + G - z$$

Newton iteration for G

```
> newtit:=subs(z=subs(vals,rho)*(1-u),G-eq/diff(eq,G));
```

$$newtit := G - \frac{-G^2 + G - 0.170391671557981 + 0.170391671557981 u}{-2 G + 1}$$

Starting point (constant coefficient):

```
> subs(vals,G);
```

$$0.217850521102698$$

Iteration:

```
> for i in newtords(nbterms) do series(subs(G=convert(%,polynom),
newtit),u,i) od;
```

$$0.217850521102697703 - 0.301952837594998 u$$

$$0.217850521102697703 - 0.301952837594997803 u + 0.161573071990073536 u^2$$

$$- 0.172913477483690 u^3 + O(u^4)$$

```
> serG:=%;
```

$$serG := 0.217850521102697703 - 0.301952837594997803 u + 0.161573071990073536 u^2$$

$$- 0.172913477483690 u^3 + O(u^4)$$

Newton iteration for B,R

```
> cc:=comp[2];
```

$$cc := [B, R]$$

```
> Sys[cc];
```

$$\left[ B - \frac{z}{1-R}, R - z^3 - \frac{z}{1-B} \right]$$

This is not as efficient as possible. In general, one would avoid the computation of an inverse. We keep this version to make the session clearer.

```
> newtit:=subs(z=subs(vals,rho)*(1-u),Vector(cc)-jac(%,cc)^(-1).
Vector(%));
```

*newtit* :=

$$\begin{bmatrix} B - \frac{(-1 \dots}{B^2 R^2 - 2 B^2 R - 2 B} \\ R - \frac{(-1 \dots}{B^2} \end{bmatrix}$$

```
> subs(vals,Vector(cc));
```

$$\begin{bmatrix} 0.219355734219891 \\ 0.223217609678837 \end{bmatrix}$$

```
> for i in newtords(nbterms) do map(series,subs(B=convert(%[1],
polynom),R=convert(%[2],polynom),newtit),u,i) od;
```

$$0.219355734219891213 - 0.309631846483247 u + O(u^2)$$

$$0.223217609678837164 - 0.319685712900192 u + O(u^2)$$

$$0.219355734219891185 - 0.309631846483246764 u + 0.179975153851467451 u^2$$

$$0.223217609678837192 - 0.319685712900192043 u + 0.186075156743548298 u^2$$

```
> serB:=%[1];serR:=%[2];
```

$$\begin{aligned} \text{serB} := & 0.219355734219891185 - 0.309631846483246764 u + 0.179975153851467451 u^2 \\ & - 0.204836305849531 u^3 + O(u^4) \end{aligned}$$

$$\begin{aligned} \text{serR} := & 0.223217609678837192 - 0.319685712900192043 u + 0.186075156743548298 u^2 \\ & - 0.200418537989039 u^3 + O(u^4) \end{aligned}$$

## Expansion of Tr,Tb,Tg

### *Implicit function theorem on the first coordinates*

Give weight 2 to u (=v^2) and 1 to Tg-Tg(rho)

This implies doubling the order of the expansions:

```
> Order:=2*nbterms;
```

$$\text{Order} := 8$$

```
> cc:=comp[3];
```

$$\text{cc} := [Tr, Tb, Tg]$$

```
> subs(z=rho*(1-v^2),Sys[cc][1..2]);
```

$$\left[ Tr - \rho (-v^2 + 1) - \frac{R}{1 - Tb}, Tb - \frac{B}{1 - Tg} \right]$$

Introduce the unknown series dTg as (Tg-Tg(rho))/v:

```
> subs(Tg=Tgrho+v*dTg,%);
```

$$\left[ Tr - \rho (-v^2 + 1) - \frac{R}{1 - Tb}, Tb - \frac{B}{-v dTg - Tgrho + 1} \right]$$

```
> jac(%,[Tr,Tb]);
```

$$\begin{bmatrix} 1 & -\frac{R}{(1-Tb)^2} \\ 0 & 1 \end{bmatrix}$$

Newton iteration for the first two coordinates in terms of v, with dTg as a parameter:

```
> newtit:=map(convert,map(series,subs(B=convert(serB,polynomial),R=
convert(serR,polynomial),rho=subs(vals,rho),Tgrho=subs(vals,Tg),u=v^2,
Vector([Tr,Tb])-%^(-1).Vector(%)),v),polynom);
```

```
newtit :=
```

$$\begin{bmatrix} \dots \\ \dots \end{bmatrix}$$

```
> Vector(subs(vals,[Tr,Tb]));
```

$$\begin{bmatrix} 0.588633437777371 \\ 0.466295268173319 \end{bmatrix}$$

```
> for i in newtords(Order) do map(series,subs(Tr=convert(%[1],
polynom),Tb=convert(%[2],polynom),newtit),v,i) od;
```

$$\begin{bmatrix} 0.588633437777371538 + 0.776782390321170 \, dTg \, v + O(v^2) \\ 0.466295268173319344 + 0.991226775511899 \, dTg \, v + O(v^2) \end{bmatrix}$$

$$\begin{bmatrix} 0.5886334377 \dots \\ \dots \\ \dots \\ \dots \end{bmatrix}$$

```
> STrTb:=%:
```

Inject those expansions into the last equation:

```
> eqsTg:=subs(Tr=STrTb[1],Tb=STrTb[2],Tg=Tgrho+v*dTg,Tgrho=subs(vals,
Tg),G=subs(u=v^2,convert(serG,polynomial)),Tg=subs(gfsys,Tg));
```

```
expand wrt v
```

```
> map(expand,series(eqsTg,v));
```

$$\begin{aligned}
& -1.42108547152020037 \times 10^{-14} dTg v + (2.38852627544253204 \\
& - 5.87130337639754529 dTg^2) v^2 + (12.9446934010627288 dTg \\
& - 34.4722033376967261 dTg^3) v^3 + (-10.4597093693150054 + 96.8410672447396905 dTg^2 \\
& - 202.396763848478685 dTg^4) v^4 + (690.934467110378819 dTg^3 \\
& - 1188.33280295549253 dTg^5 - 105.748105243046439 dTg) v^5 + ( \\
& -990.099261384640045 dTg^2 + 4775.04677772891500 dTg^4 - 6977.06239827644458 dTg^6 \\
& + 50.0102320247011960) v^6 + (-40964.4500163363 dTg^7 - 8415.23355428782 dTg^3 \\
& + 32253.4630938194 dTg^5 + 723.114084778149 dTg) v^7 + O(v^8)
\end{aligned}$$

The coefficient of  $v^0$  and  $v^1$  are expected to be 0; discard them

```
> series((%-coeff(%,v,0)-coeff(%,v,1)*v)/v^2,v);
```

$$\begin{aligned}
& 2.38852627544253204 - 5.87130337639754529 dTg^2 + (12.9446934010627288 dTg \\
& - 34.4722033376967261 dTg^3) v + (-10.4597093693150054 + 96.8410672447396905 dTg^2 \\
& - 202.396763848478685 dTg^4) v^2 + (690.934467110378819 dTg^3 \\
& - 1188.33280295549253 dTg^5 - 105.748105243046439 dTg) v^3 + ( \\
& -990.099261384640045 dTg^2 + 4775.04677772891500 dTg^4 - 6977.06239827644458 dTg^6 \\
& + 50.0102320247011960) v^4 + (-40964.4500163363 dTg^7 - 8415.23355428782 dTg^3 \\
& + 32253.4630938194 dTg^5 + 723.114084778149 dTg) v^5 + O(v^6)
\end{aligned}$$

Now, solve this equation in dTg as a power series in v (again by Newton iteration), taking for constant term the negative solution:

```
> eqdTg:=convert(%,polynom):
> newtit:=dTg-eqdTg/diff(eqdTg,dTg):
> solve(coeff(eqdTg,v,0),dTg);
      -0.6378194385, 0.6378194385
> select(type,[%],negative);
      [-0.6378194385]
> op(%):
> for i in newtords(Order-2) do series(subs(dTg=convert(%,polynom),
newtit),v,i) od;
      -0.637819438532583605 - 0.0918934790164518 v + O(v^2)
      -0.637819438510276893 - 0.0918934787882779297 v + 0.258036086531522 v^2 + O(v^3)
-0.637819438510276782 - 0.0918934787882780268 v + 0.258036086540546439 v^2
      + 0.136957918975608994 v^3 - 0.263221621178375165 v^4 - 0.176404239197979 v^5 + O(v^6)
> serdTg:=%:
> serTg:=series(subs(v=u^(1/2),series(subs(vals,Tg)+v*serdTg,v)),u);
serTg := 0.529577610600248 - 0.637819438510277 sqrt(u) - 0.0918934787882780 u
      + 0.258036086540546 u^3/2 + 0.136957918975609 u^2 - 0.263221621178375 u^5/2
      - 0.176404239197979 u^3 + O(u^7/2)
```

Substitute back into the series expansions for Tr and Tb

```
> map(series,subs(v=u^(1/2),map(series,subs(dTg=serdTg,map(convert,
STrTb,polynom)),v)),u);
```

$$0.588633437777372 - 0.495446908039319 \sqrt{u} \cdots$$

$$0.466295268173319 - 0.632223705393351 \cdots$$

```
> serTr:=%[1];serTb:=%%[2];
```

$$\begin{aligned} \text{serTr} := & 0.588633437777372 - 0.495446908039319 \sqrt{u} - 0.0979171598726323 u \\ & - 0.00346387380967139 u^3 / 2 + 0.0215317695023420 u^2 - 0.00329311780859509 u^5 / 2 \\ & - 0.0299920473184567 u^3 + O(u^7 / 2) \end{aligned}$$

$$\begin{aligned} \text{serTb} := & 0.466295268173319 - 0.632223705393351 \sqrt{u} + 0.107909889309139 u \\ & + 0.232963437313864 u^3 / 2 - 0.165390451236192 u^2 - 0.207050030048214 u^5 / 2 \\ & + 0.215706370431832 u^3 + O(u^7 / 2) \end{aligned}$$

### Formula of Prop. 8.2

This is not necessary for the rest of the calculation. It explains the notation in that proposition and will recover the same coefficients of sqrt(u) as above.

*Left and right eigenvectors of the Jacobian matrix*

```
> Jac:=J[-3..-1,-3..-1];
```

$$\text{Jac} := \begin{bmatrix} 1 & -\frac{R}{(1 - Tb)^2} & 0 \\ 0 & 1 & -\frac{B}{(1 - Tg)^2} \\ -\frac{G}{(1 - Tr)^2} & 0 & 1 \end{bmatrix}$$

```
> chareq:=collect(LinearAlgebra[Determinant](Jac),G,factor);
```

$$\text{chareq} := 1 - \frac{B R G}{(-1 + Tr)^2 (-1 + Tb)^2 (-1 + Tg)^2}$$

```
> cw:=[seq(w[j],j=1..3)]:ww:=Vector(cw); sysW:=convert(Jac.ww,list);
```

$$ww := \begin{bmatrix} w_1 \\ w_2 \\ w_3 \end{bmatrix}$$

$$sysW := \left[ w_1 - \frac{R w_2}{(1 - Tb)^2}, w_2 - \frac{B w_3}{(1 - Tg)^2}, -\frac{G w_1}{(1 - Tr)^2} + w_3 \right]$$

> solve([op(sysW[1..2]),w[2]=1],cw)[1];

$$\left[ w_1 = \frac{R}{Tb^2 - 2 Tb + 1}, w_2 = 1, w_3 = \frac{Tg^2 - 2 Tg + 1}{B} \right]$$

> solW:=factor(%);

$$solW := \left[ w_1 = \frac{R}{(-1 + Tb)^2}, w_2 = 1, w_3 = \frac{(-1 + Tg)^2}{B} \right]$$

This is a solution since

> subs(solW,sysW[3]);

$$-\frac{G R}{(1 - Tr)^2 (-1 + Tb)^2} + \frac{(-1 + Tg)^2}{B}$$

> cv:=[seq(v[j],j=1..3)]:vv:=Vector[row](cv); sysV:=convert(vv.Jac,  
list);

$$vv := \begin{bmatrix} v_1 & v_2 & v_3 \end{bmatrix}$$

$$sysV := \left[ v_1 - \frac{v_3 G}{(1 - Tr)^2}, -\frac{v_1 R}{(1 - Tb)^2} + v_2, -\frac{v_2 B}{(1 - Tg)^2} + v_3 \right]$$

> solve([op(sysV[1..2]),v[3]=1],cv)[1];

$$\left[ v_1 = \frac{G}{Tr^2 - 2 Tr + 1}, v_2 = \frac{R G}{Tb^2 Tr^2 - 2 Tb^2 Tr - 2 Tb Tr^2 + Tb^2 + 4 Tb Tr + Tr^2 - 2 Tb - 2 Tr + 1}, v_3 = 1 \right]$$

> solV:=factor(%);

$$solV := \left[ v_1 = \frac{G}{(-1 + Tr)^2}, v_2 = \frac{R G}{(-1 + Tb)^2 (-1 + Tr)^2}, v_3 = 1 \right]$$

> solV:=subs(isolate(chareq,R),solV);

$$solV := \left[ v_1 = \frac{G}{(-1 + Tr)^2}, v_2 = \frac{(-1 + Tg)^2}{B}, v_3 = 1 \right]$$

This is a solution since

> normal(subs(solV,sysV[3]));

Coefficient of  $\sqrt{1-z/\rho}$

```
> T:=Vector([seq(c[i,1],i=[G,B,R])]);
```

$$T := \begin{bmatrix} c_{G,1} \\ c_{B,1} \\ c_{R,1} \end{bmatrix}$$

```
> H:=subs(gfsys,[Tr,Tb,Tg]);
```

$$H := \left[ z + \frac{R}{1 - Tb}, \frac{B}{1 - Tg}, \frac{G}{1 - Tr} \right]$$

```
> W:=-jac(H,[G,B,R]).T+z*Vector(map(diff,H,z));
```

$$W := \begin{bmatrix} -\frac{c_{R,1}}{1 - Tb} + z \\ -\frac{c_{B,1}}{1 - Tg} \\ -\frac{c_{G,1}}{1 - Tr} \end{bmatrix}$$

```
> numer_sqrt:=2*subs(solV,vv).W;
```

$$\text{numer\_sqrt} := \frac{2 G \left( -\frac{c_{R,1}}{1 - Tb} + z \right)}{(-1 + Tr)^2} - \frac{2 (-1 + Tg)^2 c_{B,1}}{B (1 - Tg)} - \frac{2 c_{G,1}}{1 - Tr}$$

```
> Hess:=[seq(VectorCalculus['Hessian'](eq,[Tr,Tb,Tg]),eq=H)];
```

$$\text{Hess} := \left[ \begin{bmatrix} 0 & 0 & 0 \\ 0 & \frac{2 R}{(1 - Tb)^3} & 0 \\ 0 & 0 & 0 \end{bmatrix}, \begin{bmatrix} 0 & 0 & 0 \\ 0 & 0 & 0 \\ 0 & 0 & \frac{2 B}{(1 - Tg)^3} \end{bmatrix} \right],$$

$$\begin{bmatrix} \frac{2G}{(1-Tr)^3} & 0 & 0 \\ 0 & 0 & 0 \\ 0 & 0 & 0 \end{bmatrix}$$

> Vector([seq(LinearAlgebra[Transpose](ww).hh.ww,hh=%)])

$$\begin{bmatrix} \frac{2w_2^2 R}{(1-Tb)^3} \\ \frac{2w_3^2 B}{(1-Tg)^3} \\ \frac{2w_1^2 G}{(1-Tr)^3} \end{bmatrix}$$

> denom\_sqrt:=vv.%;

$$denom\_sqrt := \frac{2v_1 w_2^2 R}{(1-Tb)^3} + \frac{2v_2 w_3^2 B}{(1-Tg)^3} + \frac{2v_3 w_1^2 G}{(1-Tr)^3}$$

> mu:=sqrt(numer\_sqrt/denom\_sqrt);

$$\mu := \sqrt{\frac{\frac{2G \left( -\frac{c_{R,1}}{1-Tb} + z \right)}{(-1+Tr)^2} - \frac{2(-1+Tg)^2 c_{B,1}}{B(1-Tg)} - \frac{2c_{G,1}}{1-Tr}}{\frac{2v_1 w_2^2 R}{(1-Tb)^3} + \frac{2v_2 w_3^2 B}{(1-Tg)^3} + \frac{2v_3 w_1^2 G}{(1-Tr)^3}}}$$

> valc:= [seq(c[i,1]=coeff(ser||i,u,1),i=[G,B,R])];

$$valc := [c_{G,1} = -0.301952837594998, c_{B,1} = -0.309631846483247, c_{R,1} = -0.319685712900192]$$

> C:=subs(valc,solV,solW,z=rho,vals,mu\*subs(solW,ww));

$$C := \begin{bmatrix} 0.495446908039320 \\ 0.632223705393352 \\ 0.637819438510277 \end{bmatrix}$$

Comparison with the previous version:

> map(coeff,map(series,subs(u=V^2,[serTr,serTb,serTg]),V),V,1)

**assuming  $V>0$ ;**

$[-0.495446908039319, -0.632223705393351, -0.637819438510277]$

## Asymptotic behaviour of the coefficients of F (Example 27)

**> serTr;**

$0.588633437777372 - 0.495446908039319 \sqrt{u} - 0.0979171598726323 u$   
 $- 0.00346387380967139 u^3 / 2 + 0.0215317695023420 u^2 - 0.00329311780859509 u^5 / 2$   
 $- 0.0299920473184567 u^3 + O(u^7 / 2)$

**> MultiSeries:-series(exp(serTr),u);**

$1.80152483667951 - 0.892559910088904 \sqrt{u} + 0.0447078283990347 u$   
 $+ 0.0446409144603203 u^3 / 2 + 0.0333906711574107 u^2 - 0.0264573718683633 u^5 / 2$   
 $- 0.0499226895584548 u^3 + O(u^7 / 2)$

Changing u into  $v^2$  simplifies the extraction of coefficients

**> series(subs(u=v^2,%),v) assuming v>0;**

$1.80152483667951224 - 0.892559910088904340 v + 0.0447078283990346922 v^2$   
 $+ 0.0446409144603202787 v^3 + 0.0333906711574107479 v^4 - 0.0264573718683632601 v^5$   
 $- 0.0499226895584548 v^6 + O(v^7)$

**> K:=ceil((op(-1,%)-1)/2);**

$K := 3$

**> add(coeff(%,v,2\*i-1)\*GAMMA(n-(2\*i-1)/2)/GAMMA(-(2\*i-1)/2),i=1..K);**

$0.251786501960928 \Gamma\left(n - \frac{1}{2}\right) + 0.0188894542023204 \Gamma\left(n - \frac{3}{2}\right) + 0.0279880755279684 \Gamma\left(n - \frac{5}{2}\right)$

**> MultiSeries:-asympt(%/GAMMA(n+1),n,K);**

$0.251786501770414 \left(\frac{1}{n}\right)^{3/2} + 0.113309392324717 \left(\frac{1}{n}\right)^{5/2} + 0.112582853225714 \left(\frac{1}{n}\right)^{7/2}$   
 $+ O\left(\left(\frac{1}{n}\right)^{9/2}\right)$

**> as:=%:**

**> for i to K do asympt\_co[i]:=subs(vals,rho)^(-n)\*convert(asympt(as+(1/n^(i+1)),n),polynom) od;**

$asympt\_co_1 := 0.251786501770414 0.170391671557981^{-n} \left(\frac{1}{n}\right)^{3/2}$

$asympt\_co_2 := 0.170391671557981^{-n} \left(0.251786501770414 \left(\frac{1}{n}\right)^{3/2}\right)$

$$+ 0.113309392324717 \left( \frac{1}{n} \right)^{5/2}$$

$$\text{asympt\_co}_3 := 0.170391671557981^{-n} \left( 0.251786501770414 \left( \frac{1}{n} \right)^{3/2} \right.$$

$$\left. + 0.113309392324717 \left( \frac{1}{n} \right)^{5/2} + 0.112582853225714 \left( \frac{1}{n} \right)^{7/2} \right)$$

Compare with high order coefficients of the generating functions, obtained using NewtonGF  
[SeriesNewtonIteration]:

```
> pp:=SeriesNewtonIteration({op(combsys)},labelled,z);
                               pp := proc(prec::posint) ... end proc

> pp(10);
[ Z = z + O(z10), G = z + z2 + 2 z3 + 5 z4 + 14 z5 + 42 z6 + 132 z7 + 429 z8 + 1430 z9 + O(z10), B
= z + z2 + 2 z3 + 6 z4 + 16 z5 + 48 z6 + 153 z7 + 502 z8 + 1694 z9 + O(z10), R = z + z2 + 3 z3
+ 5 z4 + 15 z5 + 46 z6 + 147 z7 + 486 z8 + 1646 z9 + O(z10), Tb = z + 2 z2 + 7 z3 + 29 z4
+ 124 z5 + 559 z6 + 2608 z7 + 12486 z8 + 61059 z9 + O(z10), Tg = z + 3 z2 + 10 z3 + 38 z4
+ 154 z5 + 660 z6 + 2959 z7 + 13749 z8 + 65750 z9 + O(z10), Tr = 2 z + 2 z2 + 7 z3 + 23 z4
+ 95 z5 + 418 z6 + 1926 z7 + 9174 z8 + 44820 z9 + O(z10), F = 1 + 2 z + 4 z2 +  $\frac{37}{3}$  z3
+  $\frac{131}{3}$  z4 +  $\frac{2639}{15}$  z5 +  $\frac{69173}{90}$  z6 +  $\frac{1111076}{315}$  z7 +  $\frac{10559357}{630}$  z8 +  $\frac{463505219}{5670}$  z9 +
O(z10) ]

> S100:=subs(pp(101),F):
> coeff(S100,z,10);

$$\frac{5767537729}{14175}$$


> evalf(%);
406880.9685

> seq(evalf(eval(asympt_co[i],n=10)),i=1..K);
385965.787402649, 403335.085804754, 405060.878461937

> seq(coeff(S100,z,10)/evalf(eval(asympt_co[i],n=10))-1,i=1..K);
0.0541892100702872, 0.00879140659019484, 0.00449337413459805

> seq(coeff(S100,z,100)/evalf(eval(asympt_co[i],n=100))-1,i=1..K);
0.00454653276166850, 0.0000461081553047027, 1.59478635741728 × 10-6

> cols:=[black,blue,red$(K-2)];
```

```
cols := [black, blue, red]
```

Ratio between the exact values and the approximations obtained by the first 3 terms of the asymptotic expansion:

```
> for i to K do pl[i]:=plots[listplot]([seq(coeff(S100,z,j)/eval
  (asympt_co[i],n=j),j=2..100)],color=cols[i]) od:
> plots[display](seq(pl[i],i=1..K));
```

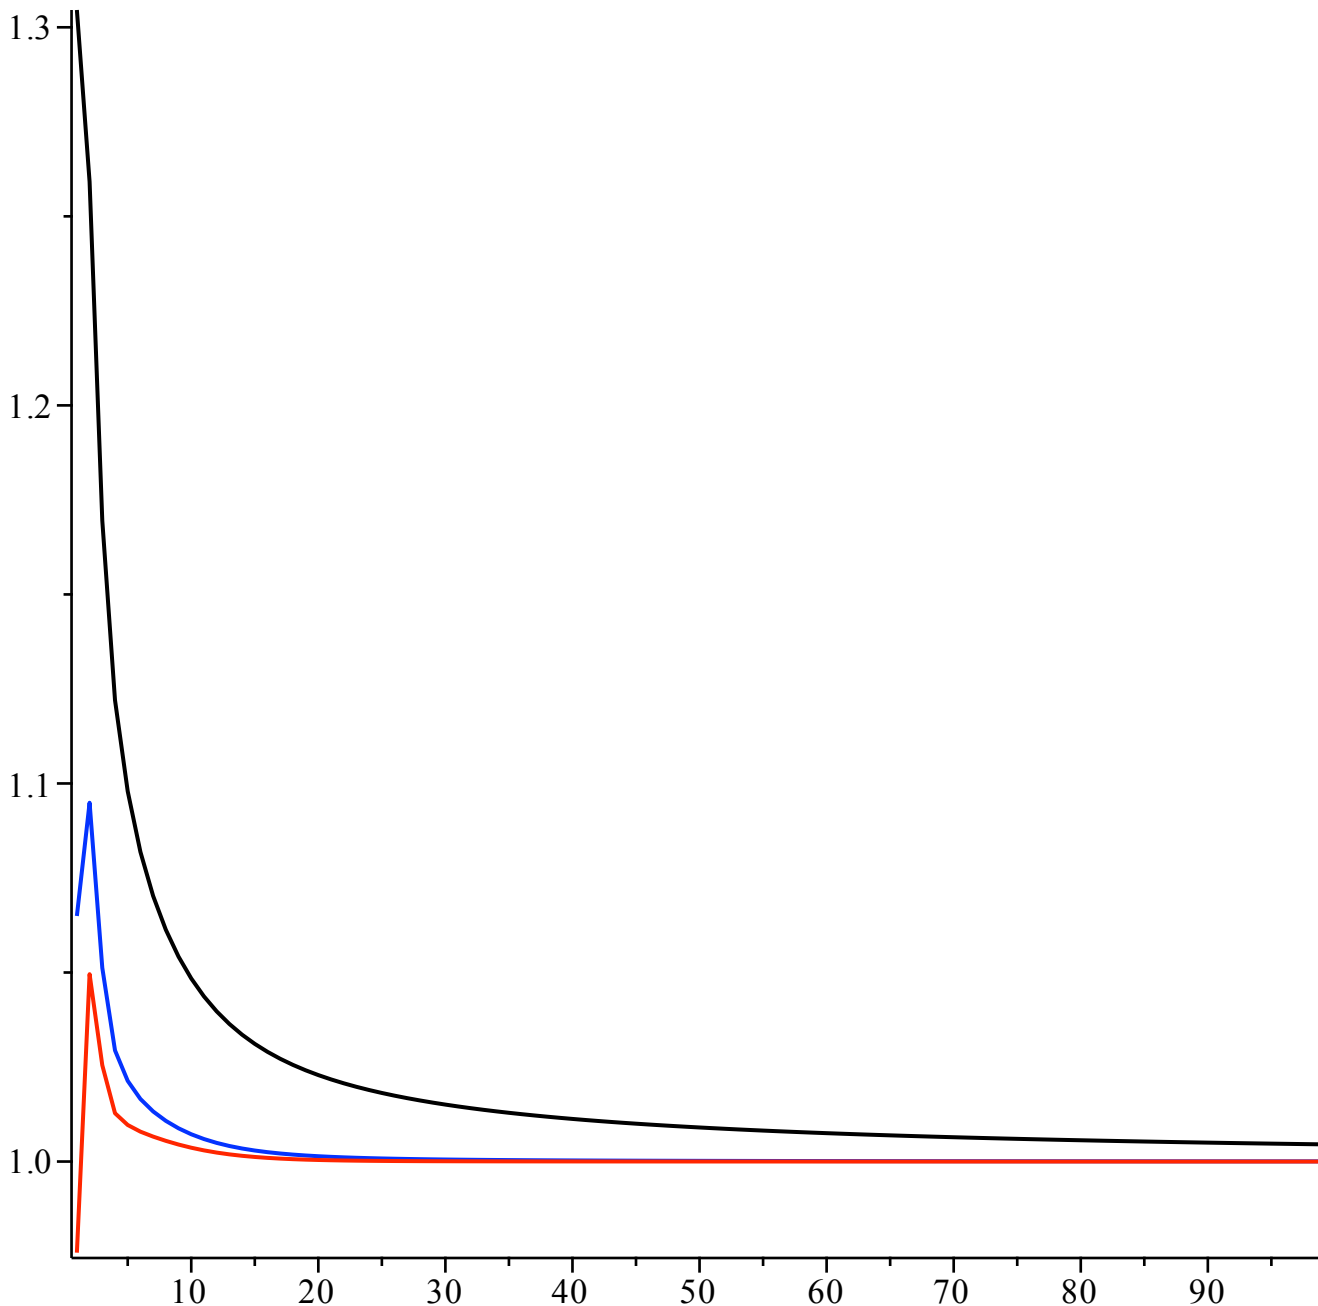

## Expected number of trees in a forest (Conclusion)

```
> num:=MultiSeries:-series(serTr*exp(serTr),u);
```

```
num := 1.06043775785598 - 1.41795051838680  $\sqrt{u}$  + 0.292132374971820 u
```

$$+ 0.0852834563116806 u^{3/2} + 0.0350417313630077 u^2 - 0.0617940001470373 u^{5/2} \\ - 0.0698315660271491 u^3 + O(u^{7/2})$$

**> series(subs(u=v^2,%),v) assuming v>0; # simplifies the extraction of coefficients**

$$1.06043775785597916 - 1.41795051838679775 v + 0.292132374971819597 v^2 \\ + 0.0852834563116805638 v^3 + 0.0350417313630077415 v^4 - 0.0617940001470372938 v^5 \\ - 0.0698315660271491 v^6 + O(v^7)$$

**> add(coeff(%,v,2\*i-1)\*GAMMA(n-(2\*i-1)/2)/GAMMA(-(2\*i-1)/2),i=1..K);**

$$0.399996456196128 \Gamma\left(n - \frac{1}{2}\right) + 0.0360870282719456 \Gamma\left(n - \frac{3}{2}\right) + 0.0653691210107923 \Gamma\left(n - \frac{5}{2}\right)$$

**> MultiSeries:-asympt(%/GAMMA(n+1),n,K);**

$$0.399996455893471 \left(\frac{1}{n}\right)^{3/2} + 0.186085699161456 \left(\frac{1}{n}\right)^{5/2} + 0.211156606691704 \left(\frac{1}{n}\right)^{7/2} \\ + O\left(\left(\frac{1}{n}\right)^{9/2}\right)$$

Note that this is really 0.399996455893471 and not a poorly approximated 0.4

**> as\_num:=%:**

**> asympt(as\_num/as,n);**

$$1.58863343777737 + \frac{0.0241419204660877}{n} + \frac{0.117433678896532}{n^2} + O\left(\frac{1}{n^3}\right)$$
